# Supplementary material for: Efficiency-Risk Tradeoffs in Dynamic Oligopoly Markets - with application to electricity markets
Source: arXiv:1209.0229 source file (2013-09-30)
Supplement: Supplementary file 1 [file appendix_old1.tex]

\begin{appendix}
  \section*{Appendix A: Linear  optimal stationary cooperative strategy}
  We postulate the value function to be of quadratic form $ V^c(x) = A^cx^2 + B^cx$ , and plug
  it in the R.H.S. of the Bellman equation in (\ref{eq:bellman2}). Solve the minimization
  problem to get the optimal strategy:
  \begin{align*}
    u^c(x,d_2) = &-\frac{1}{1+A^c}x + \frac{A^c}{1+A^c}d_2
    % \\&
    + \frac{A^c}{1+A^c}\mu_1 + \frac{B^c}{2(1+A^c)}
  \end{align*}
  Substituting back in the R.H.S., and matching terms on both sides yield the coefficients
  $A^c$, $B^c$, and the optimal per period cost $\lambda^c $:
  \begin{align*}
    \lambda^c =& A^c\sigma_1^2 + \frac{A^c}{1+A^c}q\sigma_2^2
    % \\&
    + \mu_1^2 + \frac{1+A^c-(A^c)^2}{1+A^c}q\mu_1^2 + 2q\mu_1\mu_2
  \end{align*}
  where
  \[ A^c = \sqrt{1-q}, \quad\quad B^c = 2(1-\sqrt{1-q})(\mu_2 + \mu_1)\].  Therefore,
  $(\lambda^c, V^c(x) = A^cx^2 + B^c x)$ forms a solution to the Bellman equation, with the
  linear optimal stationary  strategy $u^c(x,d_2)$ in (\ref{eq:2-linear-policy}).
  

\section*{Appendix B: Upperbound on Risk for $L=2$}
Under the assumption that $\mathcal D_i\sim\mathcal N(\mu_i,\sigma_i^2), \ i\in\{1,2\}$ the
load distributions are normal, $\{\mathcal X_k:k\}$ are correlated normal random
variables. Note that the mean and variance of $\mathcal X_k$ are both increasing in $k$, we can
upper bound the tail probability of $\mathcal X$ by the limiting distribution
$\lim_{k\to\infty}\mathcal X_k$ as follows:
\begin{align*}
  \Pr(\mathcal X\ge M)
  % &= (1-q)\sum_{k=0}^{\infty}q^k\Pr(\mathcal X_k\ge M)
  % \nonumber\\
  & <\Pr(\lim_{k\to\infty} \mathcal X_k\ge M)
\end{align*}
Since the mean and variance of the $\lim_{k\to\infty}\mathcal X_k$ equal $\lim_{k\to\infty}\mbb
E[\mathcal X_k]$ and $\lim_{k\to\infty}\text{Var}[\mathcal X_k]$, and it has normal
distribution, we have:
\begin{align*}
  \Pr(\mathcal X\ge M) = 1- \Phi\left(\frac{M-\frac{\mu_1 + (1-b)\mu_2 - e}{1-a}
    }{\frac{\sigma_1^2 + (1-b)^2\sigma_2^2}{1-a^2}}\right)
\end{align*}
and the second inequality in (\ref{eq:upperbound_X}) follows standard bound of tail probability
for normal distribution.
%\tc{red}{ We only look at the spikes that are produced by the absence of shiftable load.}
% For a general linear strategy $u(x,d_2) = -ax + bd_2 + g$, the instantaneous aggregate demand
% is given by:
% \begin{align*}
%   U(t)  =
%   x(t) + u(t)\cdot\mathbf 1[d_2(t)>0] =
%   \left\{
%     \begin{array}{ll}
%       (1-a)x(t) + bd_2(t) +e, & \text{if }  d_2(t)>0
%       \\
%       x(t), &\text{if }  d_2(t)=0
%     \end{array}
%     \right.
% \end{align*}
% Since a spike necessarily happens at time $t$ when $x(t)$ is high and $h_2(t) = 0$, as the
% aggregate demand equals $x(t)$. We can focus on the distribution of aggregate backlog state
% $x(t)$.  We denote the stationary distribution of $x(t)$ by $\mathcal X$, which is
% characterized as follows: 
% \begin{align*}
%   &\mathcal X = \mathcal X_k,\ \ \text{with probability }
%   q^k(1-q),
%   \\
%   &\mathcal X_k = \sum_{i=1}^{k} a^{i-1}\Big( \mathcal D_{1,i} + (1-b)\mathcal
%   D_{2,i}\Big) + a^k \mathcal D_{1,k} - \frac{1-a^k}{1-a} e, \ \ \forall k\ge 0
% \end{align*}
% where $\{\mathcal D_{1,i}:i\}$ and $\{\mathcal D_{2,i}:i\}$ are i.i.d. distributed random
% variables following distribution $\mathcal D_{1}$ and $\mathcal D_{2}$, respectively.  The
% mean and variance of $\mathcal X_k$  are given by:
% \begin{align*}
%   \mathbb E[\mathcal X_k] &= \frac{(1-a^{k+1})\mu_1 +
%     (1-a^{k})((1-b)\mu_2 -e)}{1-a}
%   \\
%   \text{Var}[\mathcal X_k] &= \frac{(1-a^{2(k+1)})\sigma_1^2 +
%     (1-a^{2k})(1-b)^2\sigma_2^2 }{1-a^2}
% \end{align*}

  
  \section*{Appendix C: Risk sensitive optimal strategy}
Assume the recursive cost function is of quardratic time invariant form:
\[
c(x) = r_0 + r_1 x + r_2 x^2
\]
\begin{align*}
  \mbb E[e^{-\frac{\theta}{2}c(d_2-u+d_1')}] =&
  e^{-\frac{\theta}{2}(r_0+r_1(d_2-u)+r_2(d_2-u)^2)}  \frac{1}{\sqrt{2\pi}\sigma_1}
  \int_{d_1'}
  e^{-\frac{\theta}{2}(r_1d_1'+r_2d_1'^2+2r_2(d_2-u)d_1' )}e^{-\frac{(d_1'-\mu_1)^2}{2\sigma_1^2}}
  d d_1'
  \\
  =& e^{-\frac{\theta}{2}(r_0+r_1(d_2-u)+r_2(d_2-u)^2)} 
  \frac{1}{\sqrt{\theta\sigma_1^2r_2+1}}
  e^{\frac{(\theta r_2(d_2-u)+\theta r_1/2 -\mu_1/\sigma_1^2 )^2}{2(\theta r_2 + 1/\sigma_1^2)}}
\end{align*}
\begin{align*}
  c(x) =& x^2+ \beta\left(
    r_0 + \frac{\theta\mu_1^2}{\sigma_1^2} + \frac{1}{\theta}\log(\theta\sigma_1^2r_2 + 1)
    -\frac{(\frac{\theta r_1}{2} - \frac{\mu_1}{\sigma_1^2})^2}{\theta(\theta r_2 +
      1/\sigma_1^2)}
    \right)
    \\
    & +  q\mbb E_{d_2}\left(
      2xu + u^2 + \beta r_1(d_2-u) +  \beta r_2(d_2-u)^2
      -\beta\frac{\theta r_2^2(d_2-u)^2 + (\theta r_1 -2\mu_1/\sigma_1^2)r_2(d_2-u)}{\theta r_2 + 1/\sigma_1^2}
    \right)
    \\
    =& x^2
    % + \beta\left(
  %   r_0 + \frac{\theta\mu_1^2}{\sigma_1^2} + \frac{1}{\theta}\log(\theta\sigma_1^2r_2 + 1)
  %   -\frac{(\frac{\theta r_1}{2} - \frac{\mu_1}{\sigma_1^2})^2}{\theta(\theta r_2 +
  %     1/\sigma_1^2)}
  % \right)
  % \\
  +q\left[
    \frac{\beta(r_2(\mu_2^2+\sigma_2^2)+(2\mu_1r_2+r_1)\mu_2)}{\theta\sigma_1^2r_2 + 1}
    -\frac{1}{1+\frac{\beta r_2}{\theta\sigma_1^2r_2 + 1}}
    \left(
      x^2 -\frac{\beta r_2(2\mu_1 + 2\mu_2 + \frac{r_1}{r_2})}{\theta\sigma_1^2r_2 + 1}x
      \right)
    \right]
    \\
    &+ q\mbb E_{d_2}\left[
      (1+\frac{\beta r_2}{\theta\sigma_1^2r_2 + 1})
      \left(
        u + \frac{1}{1+\frac{\beta r_2}{\theta\sigma_1^2r_2 + 1} }
      (
        x-\frac{\beta r_2}{\theta\sigma_1^2r_2 + 1} d_2
        -\frac{\beta r_2 (2\mu_1 + \frac{r_1}{2r_2})}{\theta\sigma_1^2r_2 +
          1}
        )
      \right)^2      
    \right] + C_1
\end{align*}
where $C_1$ is a constant term that does not depend on $x$. Since $u(x,d_2)$ is chosen to
minimizes the cost $c(x)$, the optimal risk sensitive load scheduling strategy is given as
follows:
\[u(x,d_2) = -\frac{1}{1+\frac{\beta r_2}{\theta\sigma_1^2r_2 + 1}} 
      (
        x-\frac{\beta r_2}{\theta\sigma_1^2r_2 + 1} d_2
        -\frac{\beta r_2 (2\mu_1 + \frac{r_1}{2r_2})}{\theta\sigma_1^2r_2 +
          1}
        )
\]
%%
Matching the above expression with the conjecture $c(x) = r_0 + r_1x + r_2 x^2$ we can obtain
$r_1$ and $r_2$ by solving the following system of equations:
\begin{align*}
  r_2 &= 1-\frac{q}{1+\frac{\beta r_2}{\theta\sigma_1^2r_2 + 1}}
  \\
  r_1 &= \frac{q}{1+\frac{\beta r_2}{\theta\sigma_1^2r_2 + 1}} \frac{\beta r_2(2\mu_1 + 2\mu_2 +
    \frac{r_1}{r_2})}{\theta\sigma_1^2r_2 + 1}
\end{align*}
% \begin{align*}
%   \left\{
%   \begin{array}{ll}
%     r_2 = 1-\frac{q}{1+\frac{\beta r_2}{\theta\sigma_1^2r_2 + 1}}
%     \\
%     r_1 = \frac{q}{1+\frac{\beta r_2}{\theta\sigma_1^2r_2 + 1}}
%     \frac{\beta r_2(2\mu_1 + 2\mu_2 + \frac{r_1}{r_2})}{\theta\sigma_1^2r_2 + 1}
%   \end{array}
% \right.
% \end{align*}

% \section*{Appendix B: Proof of efficiency upperbound}
% \[  
% - \frac{1}{2} \lambda <-\frac{\mu_2^2 + \sigma_2^2}{2}
% \exp({2\int_{-\pi}^{\pi} \log|S(e^{j\omega})| d w}) 
% \]

% \section*{Appendix C: Proof of risk upperbound}


\section*{Appendix D: Example of state space model of LTI system for $L=3$}
As an example, for $L=3$
% the LTI system dynamics are given as follows:
% \begin{align*}
%   &\mb x(t+1) = \mb R_1(\mb x(t) - \mb u(t)) + \mb R_2 \mb d(t)
%   \\
%   & \mb u(t) = \mb F \mb x(t)
% \end{align*}
 and the two outputs that we measure are:
\begin{align*}
  & y_1 = [1\ 1\ 1\ 1\ 1\ 1\ ] \mb F\mb x(t)
  \\
  & y_2 = [1\ 1\ 1\ 1\ 1\ 1\ ] \mb x(t)
\end{align*}
The constant matrices $\mb R_1$, $\mb R_2$, and $\mb F$ are given by:
  {\small
\begin{align*}
  &\mb R_1 = \left[
    \begin{array}{llllll}
      0    & 0    & 0    & 0    & 0    & 0\\
      0    & 0    & 0    & 1    & 0    & 0\\
      0    & 0    & 0    & 0    & 1    & 0\\
      0    & 0    & 0    & 0    & 0    & 0\\
      0    & 0    & 0    & 0    & 0    & 1\\
      0    & 0    & 0    & 0    & 0    & 0\\
    \end{array}
  \right],
  \ \ \ \ 
  \mb R_2 =  \left[
    \begin{array}{lll}
     1    & 0    & 0\\
     0    & 0    & 0\\
     0    & 0    & 0\\
     0    & 1    & 0\\
     0    & 0    & 0\\
     0    & 0    & 1\\
    \end{array}
  \right],
  \ \ \ \
   \mb F =  \left[
    \begin{array}{cccccc}
      1    & 0    & 0    & 0    & 0    & 0\\
      0    & 1    & 0    & 0    & 0    & 0\\
      0    & 0    & 1    & 0    & 0    & 0\\
      -\frac{\delta}{5}    & -\frac{\delta}{5}    & -\frac{\delta}{5}    & 1-\delta    & -\frac{\delta}{5}    & -\frac{\delta}{5}\\
      -\frac{\delta}{5}    & -\frac{\delta}{5}    & -\frac{\delta}{5}    & -\frac{\delta}{5}    & 1-\delta    & -\frac{\delta}{5}\\
      -\frac{\delta}{5}    & -\frac{\delta}{5}    & -\frac{\delta}{5}    & -\frac{\delta}{5}    & -\frac{\delta}{5}    & 1-\delta    \end{array}
  \right],
 \end{align*}
}

\section*{Appendix E: L2 norm of the aggregate demand and backlog}
  The problem is equivalent to showing that the two constraints in
  the following optimization problem are binding.
  \begin{align*}
    \min_{\mb P_c\in \mb R^{D_c}\times \mb R^{D_c}, \ \mb G\in \mathcal G_s}
    &\mb e'(\mb I - \mb G)\mb P_c(\mb I - \mb G)'\mb e
    \\
    \text{subject to: }& \mb e'\mb P_c\mb e \le \beta_i
    \\
    & \mb e_L'\mb G\mb P_c \mb G'\mb e_L \le \beta_j
    \\
    & \mb P_c - \mb R_1\mb G\mb P_c\mb G'\mb R_1' = \mb R_2\mb R_2'
  \end{align*}
  Then the problem is equivalent to show that:
  \begin{align*}
    &0 \prec\boldsymbol\gamma^*
    \\
   &\boldsymbol\gamma^* = \arg\max_{\boldsymbol\gamma=[\gamma_1,\gamma_2]} \Big\{
      \min_{\mb G\in\mathcal G} \mb
      e'(\mb I - \mb G)\mb P_c(\mb I - \mb G)'\mb e + \gamma_1 \mb e'\mb P_c\mb e + \gamma_2 \mb
      e_L'\mb G\mb P_c \mb G'\mb e_L
    \Big\}
  \end{align*}
  where matrix $\mb P_c$ is given by:
  \[
  \mb P_c = \sum_{\tau=0}^{\infty} (\mb R_1\mb G)^{\tau}\mb R_2\mb R_2'(\mb G'\mb R_1')^{\tau}.
  \]
  In all the classes $\mathcal G$ we consider, the elements are small, and we can approximate
  the matrix $P$ by low order moments of $\mb G$, and write the objective function as sum of
  kronecker products $\mb G$ in the vector form.
  \[\mb P_c  \approx \mb R_2\mb R_2' +  \mb R_1\mb G\mb R_2\mb R_2'\mb G'\mb R_1'\]




\section*{Appendix F: L2 norm of the aggregate demand and backlog}
%\paragraph{Approach 1}
It is very straight forward to show that with the parameterization of load scheduling strategy,
the aggregate backlog volatility $\|Y_2\|_2^2$ is increasing in $\delta$.  All we need to show
is that the aggregate demand volatility $\|Y_1\|_2^2$ is decreasing in $\delta$.  Note that
every element in $\mb R_1(\mb I-\mb F)$ is either 0 or proportional to $\delta$ with slope
smaller or equal than 1, thus for small $\delta$ less than 0.5, the first two summands in
(\ref{eq:inf-sum-M}) plays dominant role to $\|Y_1\|_2^2$. We expand it as follows:
\begin{align*}
  \|Y_1\|_2^2 =& (\mb e'\mb F\mb R_2) (\mb e'\mb F\mb R_2)' + 
   (\mb e'\mb F\mb R_1(\mb I-\mb F)\mb R_2) (\mb e'\mb F\mb R_1(\mb I-\mb F)\mb R_2)' + o(\delta^4)
  \\
   =& \left(\frac{L-1}{L+1}\right)^2 \left(\delta - \frac{L+1}{L-1}\right)^2
  + (L-1)\left(\frac{2(L-1)}{L}\right)^2 \left(\delta - \frac{L}{2(L-1)}\right)^2
  \\
  &+ \left(2\frac{L-1}{L+1} +2\frac{(L-1)(L-2)}{L(L+2)} \right)^2
  \left(\delta -
   \frac{ \frac{L-4}{L+2} }{2\frac{L-1}{L+1} +2\frac{(L-1)(L-2)}{L(L+2)}}
 \right)^2 \delta^2
 \\
  &+ \left(1+\frac{2(L-1)(L-2)}{L(L+2)}\right)^2
  \left(\delta -
   \frac{ \frac{L+1}{L-1}+\frac{L-2}{L+2} }{1+\frac{2(L-1)(L-2)}{L(L+2)}}
  \right)^2 \delta^2
 \\
  &+ (L-1)\left(\frac{2(L+1)(L-1)}{(L+2)L}\right)^2\left(\delta-\frac{L}{2(L-1)}\right)^2 \delta^2
  + o(\delta^4)
  \\
  % \stackrel{\approx}{\text{\small for L large enough \ }}
  \approx
  &2^2L\left(
    (\delta-\frac{1}{2})^2 + (\delta - \frac{2}{3})^2\delta^2
  \right)
\end{align*}
where the last approximation is accurate for $L$ large enough, and is decreasing in $\delta$
for $0<\delta<0.5$.
\\
% %\tc{blue}{Need to make sure that higher order terms are neglegible...}
% \tc{blue}{\paragraph{Approach 2}
% $\mathcal H_2$ optimization to determine feedback control $\mb F$:
% \begin{align*}
%   &\min_{\mb F} \left\| [w_1, w_2] \left[
%       \begin{array}{c}
%         \mb e' \mb F
%         \\
%         \mb e'  
%       \end{array}
%     \right] \left(z\mb I - \mb R_1 (\mb I - \mb F) \right)^{-1} \mb R_2 \mb D(z) \right\|_2
%   \\
%   &\text{subject to the deadline constraints in (\ref{eq:fb-constr-F})}
% \end{align*}
% where the positive constant $w_1$ and $w_2$ are the weight on the two output measurements.  \\
% (not sure how to proceed yet) }


\end{appendix}









%====================================================================
%====================================================================
%====================================================================
%====================================================================
%====================================================================




\begin{appendix}
  \section*{Appendix A: Linear  optimal stationary cooperative strategy}
  We postulate the value function to be of quadratic form $ V^c(x) = A^cx^2 + B^cx$ , and plug
  it in the R.H.S. of the Bellman equation in (\ref{eq:bellman2}). Solve the minimization
  problem to get the optimal strategy:
  \begin{align*}
    u^c(x,d_2) = &-\frac{1}{1+A^c}x + \frac{A^c}{1+A^c}d_2
    % \\&
    + \frac{A^c}{1+A^c}\mu_1 + \frac{B^c}{2(1+A^c)}
  \end{align*}
  Substituting back in the R.H.S., and matching terms on both sides yield the coefficients
  $A^c$, $B^c$, and the optimal per period cost $\lambda^c $:
  \begin{align*}
    \lambda^c =& A^c\sigma_1^2 + \frac{A^c}{1+A^c}q\sigma_2^2
    % \\&
    + \mu_1^2 + \frac{1+A^c-(A^c)^2}{1+A^c}q\mu_1^2 + 2q\mu_1\mu_2
  \end{align*}
  where
  \[ A^c = \sqrt{1-q}, \quad\quad B^c = 2(1-\sqrt{1-q})(\mu_2 + \mu_1)\].  Therefore,
  $(\lambda^c, V^c(x) = A^cx^2 + B^c x)$ forms a solution to the Bellman equation, with the
  linear optimal stationary  strategy $u^c(x,d_2)$ in (\ref{eq:2-linear-policy}).
  

\section*{Appendix B: Upperbound on Risk for $L=2$}
Under the assumption that $\mathcal D_i\sim\mathcal N(\mu_i,\sigma_i^2), \ i\in\{1,2\}$ the
load distributions are normal, $\{\mathcal X_k:k\}$ are correlated normal random
variables. Note that the mean and variance of $\mathcal X_k$ are both increasing in $k$, we can
upper bound the tail probability of $\mathcal X$ by the limiting distribution
$\lim_{k\to\infty}\mathcal X_k$ as follows:
\begin{align*}
  \Pr(\mathcal X\ge M)
  % &= (1-q)\sum_{k=0}^{\infty}q^k\Pr(\mathcal X_k\ge M)
  % \nonumber\\
  & <\Pr(\lim_{k\to\infty} \mathcal X_k\ge M)
\end{align*}
Since the mean and variance of the $\lim_{k\to\infty}\mathcal X_k$ equal $\lim_{k\to\infty}\mbb
E[\mathcal X_k]$ and $\lim_{k\to\infty}\text{Var}[\mathcal X_k]$, and it has normal
distribution, we have:
\begin{align*}
  \Pr(\mathcal X\ge M) = 1- \Phi\left(\frac{M-\frac{\mu_1 + (1-b)\mu_2 - e}{1-a}
    }{\frac{\sigma_1^2 + (1-b)^2\sigma_2^2}{1-a^2}}\right)
\end{align*}
and the second inequality in (\ref{eq:upperbound_X}) follows standard bound of tail probability
for normal distribution.
%\tc{red}{ We only look at the spikes that are produced by the absence of shiftable load.}
% For a general linear strategy $u(x,d_2) = -ax + bd_2 + g$, the instantaneous aggregate demand
% is given by:
% \begin{align*}
%   U(t)  =
%   x(t) + u(t)\cdot\mathbf 1[d_2(t)>0] =
%   \left\{
%     \begin{array}{ll}
%       (1-a)x(t) + bd_2(t) +e, & \text{if }  d_2(t)>0
%       \\
%       x(t), &\text{if }  d_2(t)=0
%     \end{array}
%     \right.
% \end{align*}
% Since a spike necessarily happens at time $t$ when $x(t)$ is high and $h_2(t) = 0$, as the
% aggregate demand equals $x(t)$. We can focus on the distribution of aggregate backlog state
% $x(t)$.  We denote the stationary distribution of $x(t)$ by $\mathcal X$, which is
% characterized as follows: 
% \begin{align*}
%   &\mathcal X = \mathcal X_k,\ \ \text{with probability }
%   q^k(1-q),
%   \\
%   &\mathcal X_k = \sum_{i=1}^{k} a^{i-1}\Big( \mathcal D_{1,i} + (1-b)\mathcal
%   D_{2,i}\Big) + a^k \mathcal D_{1,k} - \frac{1-a^k}{1-a} e, \ \ \forall k\ge 0
% \end{align*}
% where $\{\mathcal D_{1,i}:i\}$ and $\{\mathcal D_{2,i}:i\}$ are i.i.d. distributed random
% variables following distribution $\mathcal D_{1}$ and $\mathcal D_{2}$, respectively.  The
% mean and variance of $\mathcal X_k$  are given by:
% \begin{align*}
%   \mathbb E[\mathcal X_k] &= \frac{(1-a^{k+1})\mu_1 +
%     (1-a^{k})((1-b)\mu_2 -e)}{1-a}
%   \\
%   \text{Var}[\mathcal X_k] &= \frac{(1-a^{2(k+1)})\sigma_1^2 +
%     (1-a^{2k})(1-b)^2\sigma_2^2 }{1-a^2}
% \end{align*}

  
  \section*{Appendix C: Risk sensitive optimal strategy}
Assume the recursive cost function is of quardratic time invariant form:
\[
c(x) = r_0 + r_1 x + r_2 x^2
\]
\begin{align*}
  \mbb E[e^{-\frac{\theta}{2}c(d_2-u+d_1')}] =&
  e^{-\frac{\theta}{2}(r_0+r_1(d_2-u)+r_2(d_2-u)^2)}  \frac{1}{\sqrt{2\pi}\sigma_1}
  \int_{d_1'}
  e^{-\frac{\theta}{2}(r_1d_1'+r_2d_1'^2+2r_2(d_2-u)d_1' )}e^{-\frac{(d_1'-\mu_1)^2}{2\sigma_1^2}}
  d d_1'
  \\
  =& e^{-\frac{\theta}{2}(r_0+r_1(d_2-u)+r_2(d_2-u)^2)} 
  \frac{1}{\sqrt{\theta\sigma_1^2r_2+1}}
  e^{\frac{(\theta r_2(d_2-u)+\theta r_1/2 -\mu_1/\sigma_1^2 )^2}{2(\theta r_2 + 1/\sigma_1^2)}}
\end{align*}
\begin{align*}
  c(x) =& x^2+ \beta\left(
    r_0 + \frac{\theta\mu_1^2}{\sigma_1^2} + \frac{1}{\theta}\log(\theta\sigma_1^2r_2 + 1)
    -\frac{(\frac{\theta r_1}{2} - \frac{\mu_1}{\sigma_1^2})^2}{\theta(\theta r_2 +
      1/\sigma_1^2)}
    \right)
    \\
    & +  q\mbb E_{d_2}\left(
      2xu + u^2 + \beta r_1(d_2-u) +  \beta r_2(d_2-u)^2
      -\beta\frac{\theta r_2^2(d_2-u)^2 + (\theta r_1 -2\mu_1/\sigma_1^2)r_2(d_2-u)}{\theta r_2 + 1/\sigma_1^2}
    \right)
    \\
    =& x^2
    % + \beta\left(
  %   r_0 + \frac{\theta\mu_1^2}{\sigma_1^2} + \frac{1}{\theta}\log(\theta\sigma_1^2r_2 + 1)
  %   -\frac{(\frac{\theta r_1}{2} - \frac{\mu_1}{\sigma_1^2})^2}{\theta(\theta r_2 +
  %     1/\sigma_1^2)}
  % \right)
  % \\
  +q\left[
    \frac{\beta(r_2(\mu_2^2+\sigma_2^2)+(2\mu_1r_2+r_1)\mu_2)}{\theta\sigma_1^2r_2 + 1}
    -\frac{1}{1+\frac{\beta r_2}{\theta\sigma_1^2r_2 + 1}}
    \left(
      x^2 -\frac{\beta r_2(2\mu_1 + 2\mu_2 + \frac{r_1}{r_2})}{\theta\sigma_1^2r_2 + 1}x
      \right)
    \right]
    \\
    &+ q\mbb E_{d_2}\left[
      (1+\frac{\beta r_2}{\theta\sigma_1^2r_2 + 1})
      \left(
        u + \frac{1}{1+\frac{\beta r_2}{\theta\sigma_1^2r_2 + 1} }
      (
        x-\frac{\beta r_2}{\theta\sigma_1^2r_2 + 1} d_2
        -\frac{\beta r_2 (2\mu_1 + \frac{r_1}{2r_2})}{\theta\sigma_1^2r_2 +
          1}
        )
      \right)^2      
    \right] + C_1
\end{align*}
where $C_1$ is a constant term that does not depend on $x$. Since $u(x,d_2)$ is chosen to
minimizes the cost $c(x)$, the optimal risk sensitive load scheduling strategy is given as
follows:
\[u(x,d_2) = -\frac{1}{1+\frac{\beta r_2}{\theta\sigma_1^2r_2 + 1}} 
      (
        x-\frac{\beta r_2}{\theta\sigma_1^2r_2 + 1} d_2
        -\frac{\beta r_2 (2\mu_1 + \frac{r_1}{2r_2})}{\theta\sigma_1^2r_2 +
          1}
        )
\]
%%
Matching the above expression with the conjecture $c(x) = r_0 + r_1x + r_2 x^2$ we can obtain
$r_1$ and $r_2$ by solving the following system of equations:
\begin{align*}
  r_2 &= 1-\frac{q}{1+\frac{\beta r_2}{\theta\sigma_1^2r_2 + 1}}
  \\
  r_1 &= \frac{q}{1+\frac{\beta r_2}{\theta\sigma_1^2r_2 + 1}} \frac{\beta r_2(2\mu_1 + 2\mu_2 +
    \frac{r_1}{r_2})}{\theta\sigma_1^2r_2 + 1}
\end{align*}
% \begin{align*}
%   \left\{
%   \begin{array}{ll}
%     r_2 = 1-\frac{q}{1+\frac{\beta r_2}{\theta\sigma_1^2r_2 + 1}}
%     \\
%     r_1 = \frac{q}{1+\frac{\beta r_2}{\theta\sigma_1^2r_2 + 1}}
%     \frac{\beta r_2(2\mu_1 + 2\mu_2 + \frac{r_1}{r_2})}{\theta\sigma_1^2r_2 + 1}
%   \end{array}
% \right.
% \end{align*}

% \section*{Appendix B: Proof of efficiency upperbound}
% \[  
% - \frac{1}{2} \lambda <-\frac{\mu_2^2 + \sigma_2^2}{2}
% \exp({2\int_{-\pi}^{\pi} \log|S(e^{j\omega})| d w}) 
% \]

% \section*{Appendix C: Proof of risk upperbound}


\section*{Appendix D: Example of state space model of LTI system for $L=3$}
As an example, for $L=3$
% the LTI system dynamics are given as follows:
% \begin{align*}
%   &\mb x(t+1) = \mb R_1(\mb x(t) - \mb u(t)) + \mb R_2 \mb d(t)
%   \\
%   & \mb u(t) = \mb F \mb x(t)
% \end{align*}
 and the two outputs that we measure are:
\begin{align*}
  & y_1 = [1\ 1\ 1\ 1\ 1\ 1\ ] \mb F\mb x(t)
  \\
  & y_2 = [1\ 1\ 1\ 1\ 1\ 1\ ] \mb x(t)
\end{align*}
The constant matrices $\mb R_1$, $\mb R_2$, and $\mb F$ are given by:
  {\small
\begin{align*}
  &\mb R_1 = \left[
    \begin{array}{llllll}
      0    & 0    & 0    & 0    & 0    & 0\\
      0    & 0    & 0    & 1    & 0    & 0\\
      0    & 0    & 0    & 0    & 1    & 0\\
      0    & 0    & 0    & 0    & 0    & 0\\
      0    & 0    & 0    & 0    & 0    & 1\\
      0    & 0    & 0    & 0    & 0    & 0\\
    \end{array}
  \right],
  \ \ \ \ 
  \mb R_2 =  \left[
    \begin{array}{lll}
     1    & 0    & 0\\
     0    & 0    & 0\\
     0    & 0    & 0\\
     0    & 1    & 0\\
     0    & 0    & 0\\
     0    & 0    & 1\\
    \end{array}
  \right],
  \ \ \ \
   \mb F =  \left[
    \begin{array}{cccccc}
      1    & 0    & 0    & 0    & 0    & 0\\
      0    & 1    & 0    & 0    & 0    & 0\\
      0    & 0    & 1    & 0    & 0    & 0\\
      -\frac{\delta}{5}    & -\frac{\delta}{5}    & -\frac{\delta}{5}    & 1-\delta    & -\frac{\delta}{5}    & -\frac{\delta}{5}\\
      -\frac{\delta}{5}    & -\frac{\delta}{5}    & -\frac{\delta}{5}    & -\frac{\delta}{5}    & 1-\delta    & -\frac{\delta}{5}\\
      -\frac{\delta}{5}    & -\frac{\delta}{5}    & -\frac{\delta}{5}    & -\frac{\delta}{5}    & -\frac{\delta}{5}    & 1-\delta    \end{array}
  \right],
 \end{align*}
}


\section*{Appendix E: L2 norm of the aggregate demand and backlog}
%\paragraph{Approach 1}
It is very straight forward to show that with the parameterization of load scheduling strategy,
the aggregate backlog volatility $\|Y_2\|_2^2$ is increasing in $\delta$.  All we need to show
is that the aggregate demand volatility $\|Y_1\|_2^2$ is decreasing in $\delta$.  Note that
every element in $\mb R_1(\mb I-\mb F)$ is either 0 or proportional to $\delta$ with slope
smaller or equal than 1, thus for small $\delta$ less than 0.5, the first two summands in
(\ref{eq:inf-sum-M}) plays dominant role to $\|Y_1\|_2^2$. We expand it as follows:
\begin{align*}
  \|Y_1\|_2^2 =& (\mb e'\mb F\mb R_2) (\mb e'\mb F\mb R_2)' + 
   (\mb e'\mb F\mb R_1(\mb I-\mb F)\mb R_2) (\mb e'\mb F\mb R_1(\mb I-\mb F)\mb R_2)' + o(\delta^4)
  \\
   =& \left(\frac{L-1}{L+1}\right)^2 \left(\delta - \frac{L+1}{L-1}\right)^2
  + (L-1)\left(\frac{2(L-1)}{L}\right)^2 \left(\delta - \frac{L}{2(L-1)}\right)^2
  \\
  &+ \left(2\frac{L-1}{L+1} +2\frac{(L-1)(L-2)}{L(L+2)} \right)^2
  \left(\delta -
   \frac{ \frac{L-4}{L+2} }{2\frac{L-1}{L+1} +2\frac{(L-1)(L-2)}{L(L+2)}}
 \right)^2 \delta^2
 \\
  &+ \left(1+\frac{2(L-1)(L-2)}{L(L+2)}\right)^2
  \left(\delta -
   \frac{ \frac{L+1}{L-1}+\frac{L-2}{L+2} }{1+\frac{2(L-1)(L-2)}{L(L+2)}}
  \right)^2 \delta^2
 \\
  &+ (L-1)\left(\frac{2(L+1)(L-1)}{(L+2)L}\right)^2\left(\delta-\frac{L}{2(L-1)}\right)^2 \delta^2
  + o(\delta^4)
  \\
  % \stackrel{\approx}{\text{\small for L large enough \ }}
  \approx
  &2^2L\left(
    (\delta-\frac{1}{2})^2 + (\delta - \frac{2}{3})^2\delta^2
  \right)
\end{align*}
where the last approximation is accurate for $L$ large enough, and is decreasing in $\delta$
for $0<\delta<0.5$.
\\
% %\tc{blue}{Need to make sure that higher order terms are neglegible...}
% \tc{blue}{\paragraph{Approach 2}
% $\mathcal H_2$ optimization to determine feedback control $\mb F$:
% \begin{align*}
%   &\min_{\mb F} \left\| [w_1, w_2] \left[
%       \begin{array}{c}
%         \mb e' \mb F
%         \\
%         \mb e'  
%       \end{array}
%     \right] \left(z\mb I - \mb R_1 (\mb I - \mb F) \right)^{-1} \mb R_2 \mb D(z) \right\|_2
%   \\
%   &\text{subject to the deadline constraints in (\ref{eq:fb-constr-F})}
% \end{align*}
% where the positive constant $w_1$ and $w_2$ are the weight on the two output measurements.  \\
% (not sure how to proceed yet) }


\end{appendix}
